# Supplementary material for: Limitations of the DFT-1/2 method for covalent semiconductors and transition-metal oxides
Source: arXiv:1901.04800 ancillary file (2019-01-15)
Supplement: Supplementary file 1 [file Supplemental_Material.pdf]

# Supplemental Material for
# Limitations of the DFT–1/2 method for covalent semiconductors and transition-metal oxides

Jan Doumont, Fabien Tran, and Peter Blaha
*Institute of Materials Chemistry, Vienna University of Technology,*
*Getreidemarkt 9/165-TC, A-1060 Vienna, Austria*

TABLE S1. Experimental lattice constants (in Å) for all solids discussed.[1–7] When necessary, the positions of atoms (in internal units) are also indicated. The space group number is indicated in parenthesis. For $Cr_2O_3$, $Fe_2O_3$, MnO, FeO, CoO, NiO, and CuO the antiferromagnetic order leads to a lowering of the symmetry (second indicated space group).

| Solid | $a$ | $b$ | $c$ | $\alpha$ | $\beta$ | $\gamma$ |
|---|---|---|---|---|---|---|
| C (227) | 3.567 | 3.567 | 3.567 | 90 | 90 | 90 |
| Si (227) | 5.430 | 5.430 | 5.430 | 90 | 90 | 90 |
| Ge (227) | 5.652 | 5.652 | 5.652 | 90 | 90 | 90 |
| SiC (216) | 4.358 | 4.358 | 4.358 | 90 | 90 | 90 |
| BN (216) | 3.616 | 3.616 | 3.616 | 90 | 90 | 90 |
| BP (216) | 4.538 | 4.538 | 4.538 | 90 | 90 | 90 |
| BAs (216) | 4.777 | 4.777 | 4.777 | 90 | 90 | 90 |
| AlN (216) | 4.342 | 4.342 | 4.342 | 90 | 90 | 90 |
| AlP (216) | 5.463 | 5.463 | 5.463 | 90 | 90 | 90 |
| AlAs (216) | 5.661 | 5.661 | 5.661 | 90 | 90 | 90 |
| AlSb (216) | 6.136 | 6.136 | 6.136 | 90 | 90 | 90 |
| GaN (216) | 4.523 | 4.523 | 4.523 | 90 | 90 | 90 |
| GaP (216) | 5.451 | 5.451 | 5.451 | 90 | 90 | 90 |
| GaAs (216) | 5.648 | 5.648 | 5.648 | 90 | 90 | 90 |
| GaSb (216) | 6.096 | 6.096 | 6.096 | 90 | 90 | 90 |
| BeO (wurtzite,186) | 2.694 | 2.694 | 4.384 | 90 | 90 | 120 |
| BeS (216) | 4.863 | 4.863 | 4.863 | 90 | 90 | 90 |
| BeSe (216) | 5.148 | 5.148 | 5.148 | 90 | 90 | 90 |
| BeTe (216) | 5.627 | 5.627 | 5.627 | 90 | 90 | 90 |
| $TiO_2$ (rutile,136) | 4.594 | 4.594 | 2.959 | 90 | 90 | 90 |
| Ti(0,0,0), O(0.305,0.305,0) | | | | | | |
| $Cr_2O_3$ (167,146) | 4.953 | 4.953 | 13.588 | 90 | 90 | 120 |
| Cr(0,0,0.3475), O(0.3058,0,1/4) | | | | | | |
| $Fe_2O_3$ (167,146) | 5.035 | 5.035 | 13.747 | 90 | 90 | 120 |
| Fe(0,0,0.35534), O(0.3056,0,1/4) | | | | | | |
| MnO (225,166) | 4.445 | 4.445 | 4.445 | 90 | 90 | 90 |
| FeO (225,166) | 4.334 | 4.334 | 4.334 | 90 | 90 | 90 |
| CoO (225,166) | 4.254 | 4.254 | 4.254 | 90 | 90 | 90 |
| NiO (225,166) | 4.171 | 4.171 | 4.171 | 90 | 90 | 90 |
| $Cu_2O$ (224) | 4.267 | 4.267 | 4.267 | 90 | 90 | 90 |
| ZnO (wurtzite,186) | 3.258 | 3.258 | 5.220 | 90 | 90 | 120 |
| Zn(1/3,2/3,0), O(1/3,2/3,0.382) | | | | | | |
| CuO (15,14) | 4.684 | 3.423 | 5.129 | 90 | 99.54 | 90 |
| Cu(1/4,1/4,0), O(0,0.4184,1/4) | | | | | | |


1 ICSD, Inorganic Crystal Structure Database, http://icsd.fiz-karlsruhe.de.
2 American Mineralogist Crystal Structure Database, http://rruff.geo.arizona.edu/AMS/amcsd.php.
3 P. Villars and J. Daams, J. Alloys Compd. **197**, 177 (1993).
4 J. Heyd, J. E. Peralta, G. E. Scuseria, and R. L. Martin, J. Chem. Phys. **123**, 174101 (2005).
5 J. M. Crowley, J. Tahir-Kheli, and W. A. Goddard, III, J. Phys. Chem. Lett. **7**, 1198 (2016).
6 H. Haas and J. G. Correia, Hyperfine Interact. **198**, 133 (2010).
7 M. Nagelstraßer, H. Dröge, H.-P. Steinrück, F. Fischer, T. Litz, A. Waag, G. Landwehr, A. Fleszar, and W. Hanke, Phys. Rev. B **58**, 10394 (1998).
